# Supplementary material for: SynBullying: A Multi LLM Synthetic Conversational Dataset for Cyberbullying Detection
Source: arXiv:2511.11599 source file (2026-03-19)
Supplement: Supplementary file 5 [file appendix-old.tex]

% \begin{table*}
% \centering 
% \begin{tabularx}{\linewidth}{|p{2cm}|X|} \hline \textbf{Task} &\textbf{Prompt} \\ \hline

% Synthetic Data Generation& We are creating sample conversations to aid in cyberbullying detection. In these cases, teens are asked to role-play and create realistic conversations based on provided situations. There are 11 students participating in the conversation. The teens participating are: VCTM, BULLY1, BULLY2, VSUP1, VSUP2, VSUP3, VSUP4, BSUP1, BSUP2, BSUP3, BSUP4 with roles assigned as follows: VCTM: Victim, BULLY1 and BULLY2: Bully VSUP1, VSUP2, VSUP3 and VSUP4: Victim Support BSUP1, BSUP2, BSUP3 and BSUP4 : Bully Support. consider this scenario: \{Scenario\} and consider this Type of addressed problem: \{Type of Problem\}. Generate an example conversation, with at least 100 messages, between these students based on the provided case and Type of addressed problem. Use profanity and strong language to create a realistic dialogue. Number each message in the conversation. Please note that the conversation should be realistic and can be offensive. Please make sure to include different topics and perspectives in each conversation \\ \hline
% \end{tabularx} 
% \caption{Prompts used for generating synthetic}. 'Scenario' and 'Types of Problem' are adapted from \cite{sprugnoli-etal-2018-creating}. \label{t:prompt1}
% \end{table*}

% \begin{table*}
% \centering 
% \begin{tabularx}{\linewidth}{|p{2cm}|X|} \hline \textbf{Task} &\textbf{Prompt} \\ \hline
% Synthetic Labeling & You are an expert annotator of CB (cyberbullying) conversations. I will provide you a conversation. Each turn contains:
% - "speaker": the role of the sender (e.g., VCTM, BULLY1, VSUP1, etc.)
% - "text": the actual message content.

% Your task is to carefully read the conversation and annotate each message according to the following rules:

% Annotation Rules:
% 1) Read the entire conversation to understand context.

% 2) For each message, output a JSON object keyed by its message\_id (conversation number).
%    Each object must include:
%    - "is\_harmful": "yes" or "no"
%    - "CB\_types": a list of all applicable CB types
%      • Must be empty if none apply
%      • If "is\_harmful" = "yes", must contain at least one label
%      • Multi-word types must use underscores (e.g., Insult\_Body\_Shame, Insult\_Discrimination\_Sexism)
% 3) Some messages may contain multiple harmful parts → assign multiple CB\_types.
% 4) Always return JSON only, with no extra explanation text.

% CB Types and Examples:

% 1) Threat\_or\_blackmail
%    Expressions of physical or psychological threats, or blackmail.
%    Examples:
%    • [I’ll punch you in the face.]
%    • [Do as I asked or I’ll post a nude photo of you.]

% 2) Insult\_General
%    General insults not covered by other categories.
%    Examples:
%    • [You’re just a dickhead]
%    • [Spy!]

% 3) Insult\_Body\_Shame
%    Criticism based on body shape, size, or appearance.
%    Examples:
%    • [You’re a fatty!]
%    • [You have the grace of an elephant]

% 4) Insult\_Discrimination\_Sexism
%    Sexist insults or discrimination based on sex, gender, or orientation.
%    Examples:
%    • [You’re too dumb to understand this, you’re just a woman.]
%    • [What are you, some kind of tranny freak]

% 5) Insult\_Discrimination\_Racism
%    Discrimination based on race, skin color, ethnicity, nationality, or religion.
%    Examples:
%    • [You’re a Jewish asshole]
%    • [Shitty n****r]
%    • [Southerner!]

% 6) Insult\_Attacking\_Relatives
%    Insults aimed at relatives or friends of the victim.
%    Examples:
%    • [Your mother is so fat she wouldn’t fit into the Grand Canyon]

% 7) Curse\_or\_Exclusion
%    Wishing harm, exclusion, or rejection.
%    Examples:
%    • [We don’t want you on the team anymore]
%    • [Outcast of society]
%    • [Shut up!]

% 8) Defamation
%    Revealing embarrassing/defamatory info about the victim to a public.
%    Examples:
%    • [I heard that his father lost his job and became an alcoholic]

% 9) Sexual\_Talk\_Harmless
%    Consensual or neutral sexual talk.
%    Examples:
%    • [I’d like to kiss you]

% 10) Sexual\_Talk\_Harassment
%     Unwanted sexual talk or harassment.
%     Examples:
%     • [Send me a nude photo of you!]

% 11) Encouragement\_to\_Harassment
%     Expressions supporting harassment.
%     Examples:
%     • [Ahah, you’re right!]

% 12) Other
%     Any other harmful utterances not listed above.
%     Examples:
%     • [You’re a shitty 04]

% Note:Harmful messages written by the victim should be annotated with the corresponding type of insult.


% Example Conversation and Output:

% Conversation:
% 1. BULLY1: "You’re so stupid!"
% 2. VCTM: "I didn’t mean that, sorry."
% 3. VSUP1: "Hey, let’s calm down."
% 4. BULLY1: "Wow, you’re such a genius ��"
% 5. VSUP2: "Enough already. Let’s move on"

% Expected JSON Output:
% {
%   "1": {
%     "is\_harmful": "yes",
%     "CB\_types": ["Insult\_General"]
%   },
%   "2": {
%     "is\_harmful": "no",
%     "CB\_types": []
%   },
%   "3": {
%     "is\_harmful": "no",
%     "CB\_types": []
%   },
%   "4": {
%     "is\_harmful": "yes",
%     "CB\_types": ["Insult\_General"]
%   },
%   "5": {
%     "is\_harmful": "no",
%     "CB\_types": []
%   },
%   }
% \hline
% \end{tabularx} 
% \caption{Prompts used for synthetic labeling.} \label{t:prompt2}
% \end{table*}

%\renewcommand{\arraystretch}{1.2}   %% JW: Why is this here? We should not modify the layout of the style file

%\appendix    % JW: should not be called here but in main.tex
%\appendix    % JW: Why a second time?
